# Supplementary material for: The different flavors of extragalactic jets: the role of relativistic flow deceleration
Source: arXiv:2007.11423 source file (2020-07-22)
Supplement: Supplementary file 1 [file appendix.tex]

\appendix

%%%%%%%%%%%%%%%%%%%%%%%%%%%%%%%%%%%%%%%%%%%%%%%%%%%
\section{Appendix}
%
%
%%%%%%%%%%%%%%%%%%%%%%%%%%%%%%%%%%%%%%%%%%%%%%%%%%%
